# Supplementary material for: Design and Analysis of group-sequential clinical trials based on a modestly-weighted log-rank test in anticipation of a delayed separation of survival curves: A practical guidance
Source: arXiv:2102.05535 source file (2021-08-26)
Supplement: Supplementary file 1 [file supplementary_material.tex]

\documentclass{article}
\usepackage[utf8]{inputenc}
\usepackage{amsmath}

\title{Supplementary material}
\author{Dominic Magirr and Jos\'e L. Jim\'enez \\
Novartis Pharma A.G., Basel, Switzerland}
\date{August 2020}

\begin{document}

\maketitle



\end{document}
